# Supplementary material for: Minimalistic Attacks: How Little it Takes to Fool a Deep Reinforcement Learning Policy
Source: arXiv:1911.03849 source file (2020-10-29)
Supplement: Supplementary file 1 [file appendix.tex]

\leftline{\textbf{Appendix A: The Atari games evaluated}}
\begin{figure}[h]
\begin{subfigure}{0.15\textwidth}
    \centering
     \includegraphics[width=0.9\textwidth]{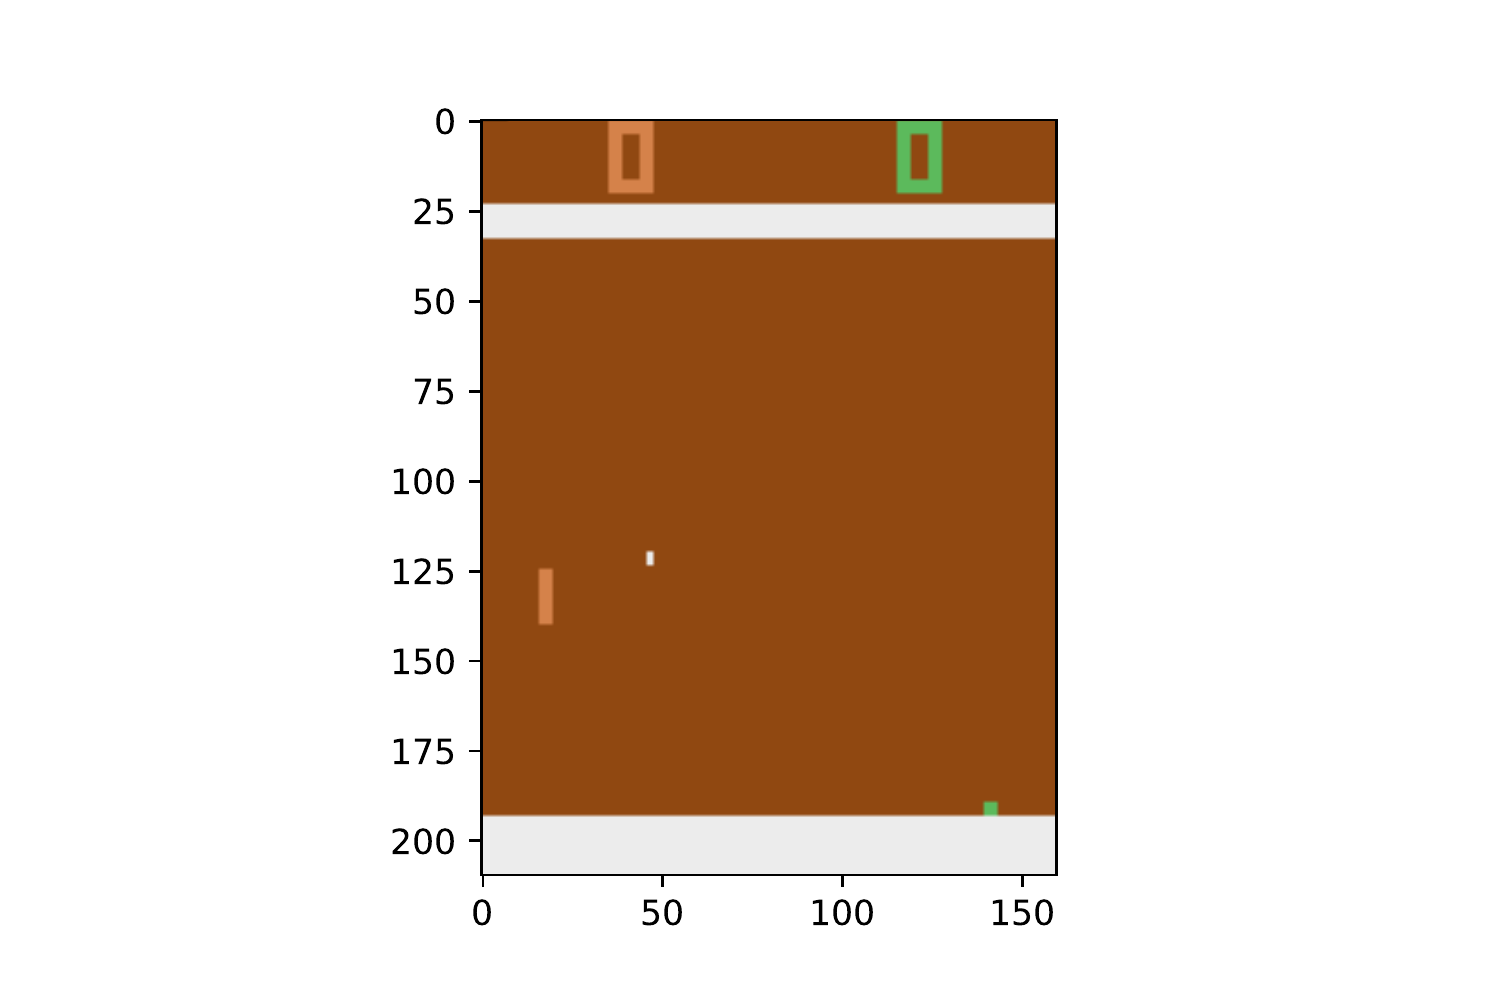}
     \caption{Pong}
\end{subfigure}
\begin{subfigure}{0.15\textwidth}
    \centering
     \includegraphics[width=0.9\textwidth]{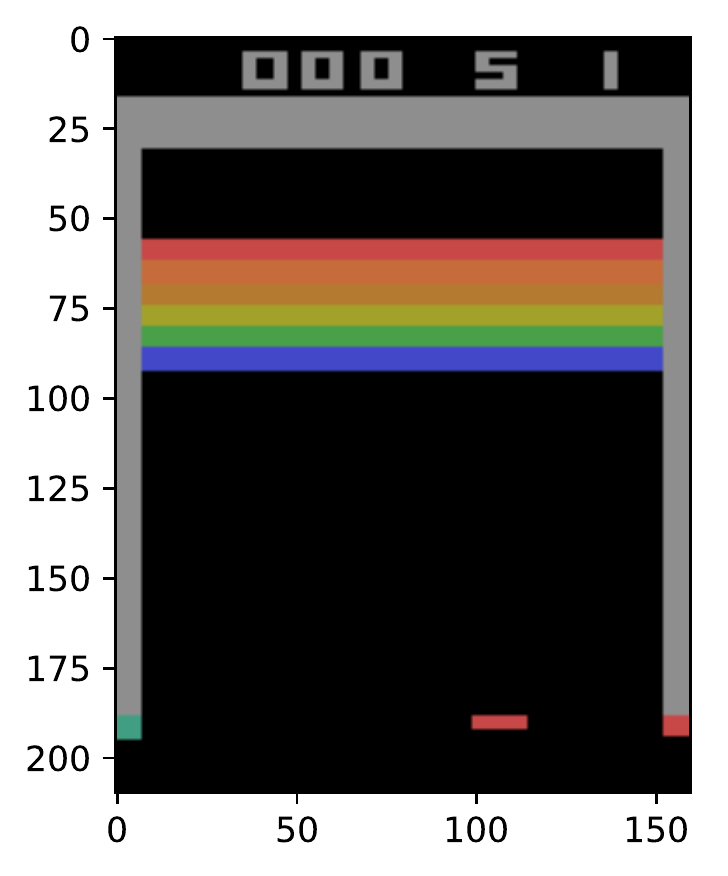}
     \caption{Breakout}
\end{subfigure}
\begin{subfigure}{0.15\textwidth}
    \centering
     \includegraphics[width=0.9\textwidth]{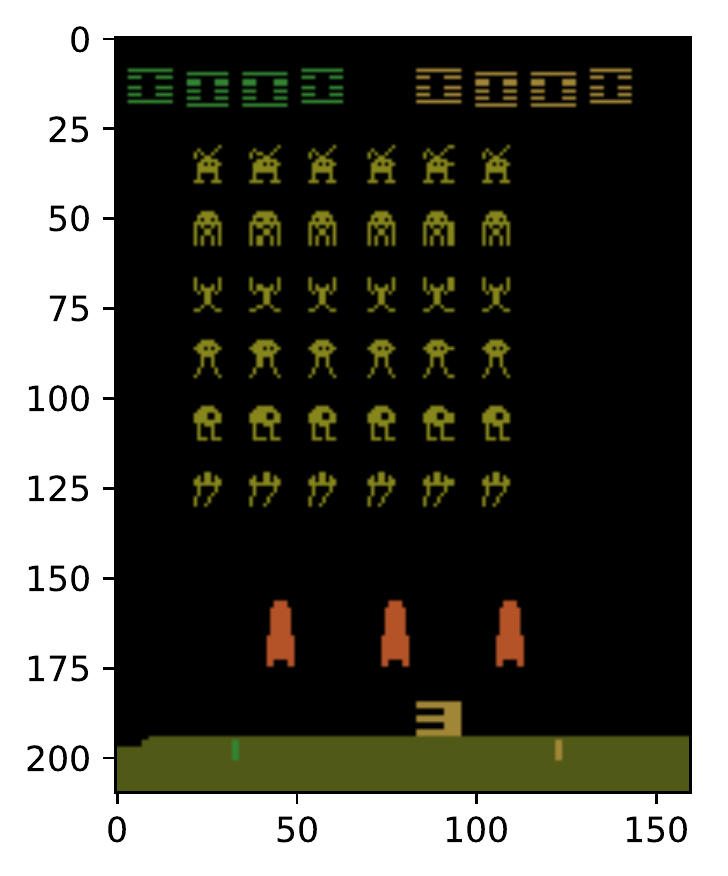}
     \caption{SpaceInvaders}
\end{subfigure}
\begin{subfigure}{0.15\textwidth}
    \centering
     \includegraphics[width=0.9\textwidth]{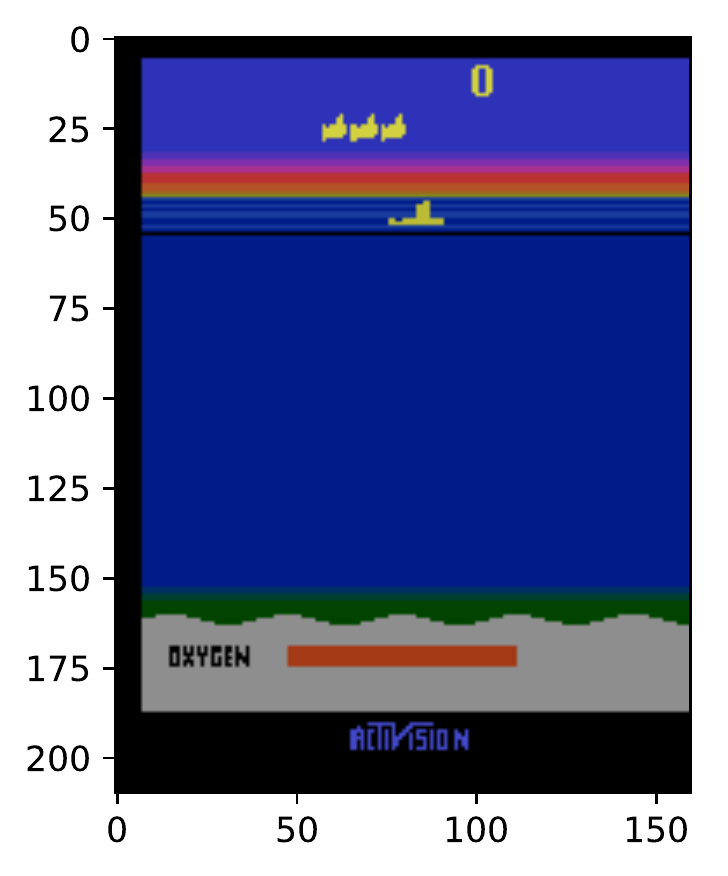}
     \caption{Seaquest}
\end{subfigure}
\hspace{0.02in}
\begin{subfigure}{0.15\textwidth}
    \centering
     \includegraphics[width=0.9\textwidth]{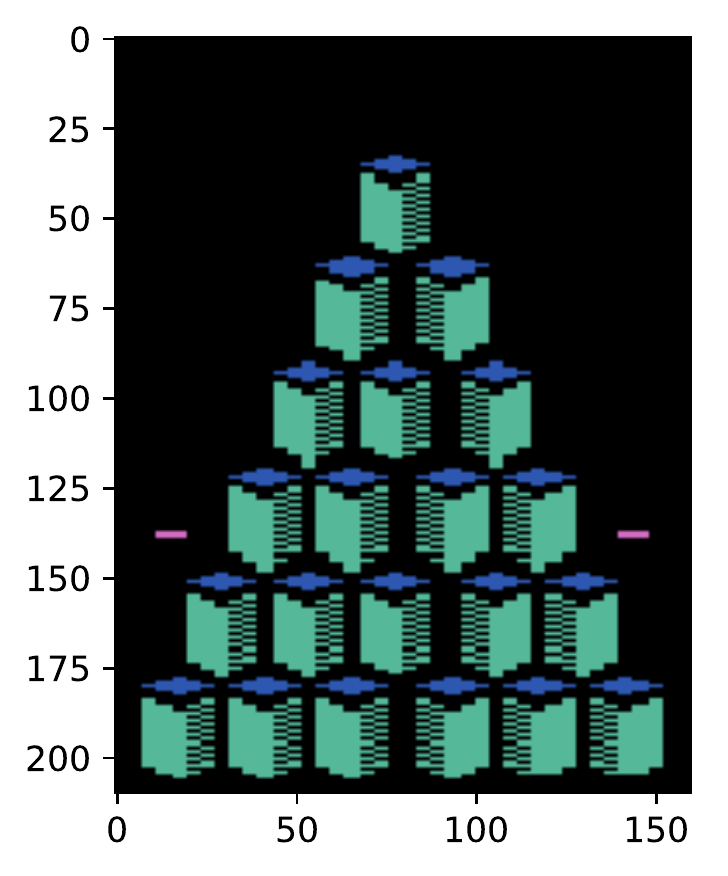}
     \caption{Qbert}
\end{subfigure}
\hspace{0.01in}
\begin{subfigure}{0.15\textwidth}
    \centering
     \includegraphics[width=0.9\textwidth]{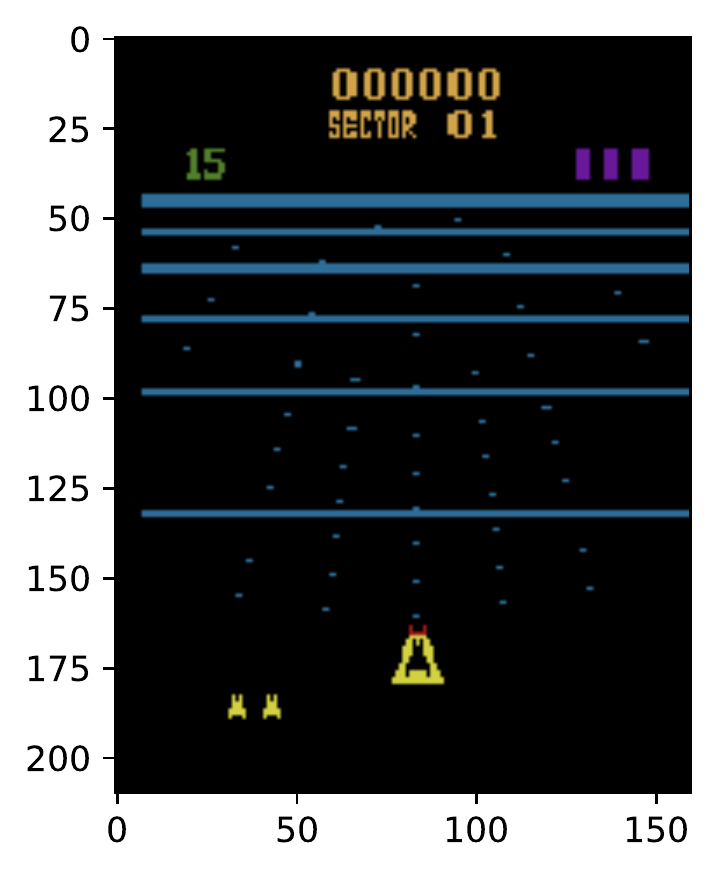}
     \caption{BeamRider}
\end{subfigure}
\caption{The six representative Atari games 
    (i.e., Pong, Breakout, SpaceInvaders, Seaquest, Qbert, BeamRider) applied in the experiments}
\label{fig:atari games}
\end{figure}
% \vspace{0.2in}
\leftline{\textbf{Appendix B: The RL algorithms evaluated}}
Reinforcement learning algorithms train a policy $\pi$ to maximize the expected cumulative reward
received. In our paper, such policy $\pi$ is a deterministic model that maps the state $s$ to a predicted action $a$. Over the past decades, many different RL algorithms have been proposed. We select several representative ones, i.e., Deep Q-Networks (DQN) \cite{mnih2013playing}, PPO \cite{schulman2017proximal}, A2C \cite{mnih2016asynchronous}, ACKTR \cite{wu2017scalable}.
\begin{itemize}[leftmargin=0.5cm]
\item \textbf{Deep Q-Networks (DQN) \cite{mnih2013playing}}: Instead of predicting the probability of each action, DQN computes the Q value for each available action. Such Q value $Q^*(s,a)$ represents the approximated expected cumulative discounted reward that obtained since the current frame. Based on such approximation, the DQN is trained via minimizing the temporal difference loss (i.e., squared Bellman error). In this paper, the corresponding policy for DQN is achieved by selecting the action with maximum Q value. In addition, to make the prediction of DQN consistent with other policies, a soft-max layer is added after the output of DQN. 

\item \textbf{Proximal Policy Optimization (PPO)\cite{schulman2017proximal}}: PPO is an off-policy  method using policy gradient, and it strikes a balance between ease of implementation, sample complexity, and ease of tuning. PPO is proposed based on trust region policy optimization (TRPO), but PPO much simpler to implement, more general, and have better sample
complexity (empirically). PPO tries to compute an update at each step with minimizing the cost function while restricting the updating step to be relatively small. To this end, in the loss function, PPO involves in a penalty term that indicates the Kullback–Leibler divergence between old policy action prediction and the new one.

\item \textbf{Advantage Actor-Critic (A2C) \cite{sutton2018reinforcement}}: A2C is an actor-critic method that learns both a policy and a state value function (i.e., also called critic). Such design is to reduce variance and accelerate learning with updating a state from subsequent estimation. The advantage $A$ means a function value that is formulated by $A = Q(s_t,a_t)-V(s_t)$, where $Q(s_t,a_t)$ is the state-action value and $V(s_t)$ is the state value. 
\item \textbf{Actor Critic using
Kronecker-Factored Trust Region (ACKTR) \cite{wu2017scalable}}: ACKTR is an extension of the natural policy gradient, and it optimizes both the actor and the critic using Kronecker-factored approximate curvature (K-FAC) with trust region. It is the first scalable trust region natural gradient method for actor-critic methods. It suggests that Kronecker-factored natural gradient approximations in reinforcement learning is a promising framework.
\end{itemize}
\vspace{0.2in}
